# Supplementary material for: Polarization properties of weakly magnetized Neutron Stars in Low Mass X-ray Binaries
Source: arXiv:2206.00749 source file (2022-06-01)
Supplement: Supplementary file 1 [file Appendix.tex]

%%%%%%%%%%%%%%%%% APPENDIX %%%%%%%%%%%%%%%%%%

Figures \ref{fig:Slab.MoreIncl} and \ref{fig:Shell.MoreIncl} show the result for the polarization degree and angle as function of energy for a LMXB in HSS respectively with a slab and a spherical shell corona observed at various viewing angles. 
We separate these viewing inclinations from those chosen in Section \ref{sec:Results} to avoid overcrowding the plots.
The behaviour of the results for different inclinations is the same as described in Section \ref{sec:Results} for both the slab and shell geometries. 

\begin{figure}
    \centering
    \includegraphics[width=0.45\textwidth]{Images/Slab_MoreIncl_Disc+NS+Direct_poldeg+ang.png}
    \caption{Polarization degree and angle as function of energy between 0.1-10 keV for a LMXB in HSS with a slab corona for different viewing inclinations. The contributions of the NS and disc seed photons scattered by the corona are summed together, considering also the disc radiation directly observed.}
    \label{fig:Slab.MoreIncl}
\end{figure}

\begin{figure}
    \centering
    \includegraphics[width=0.45\textwidth]{Images/Shell_MoreIncl_Disc+NS+Direct_poldeg+ang.png}
    \caption{Same as Figure \ref{fig:Shell.MoreIncl} but for a LMXB in HSS with a spherical shell corona.}
    % \caption{Polarization degree and angle as function of energy between 0.1-10 keV for a LMXB in HSS with a spherical shell corona for different viewing inclinations. The contributions of the NS and disc seed photons scattered by the corona are summed together, considering also the disc radiation directly observed.}
    \label{fig:Shell.MoreIncl}
\end{figure}
